# Supplementary material for: Sequential Attend, Infer, Repeat: Generative Modelling of Moving Objects
Source: arXiv:1806.01794 source file (2018-11-21)
Supplement: Supplementary file 1 [file air.tex]

\section{Details of AIR}
